# Supplementary material for: BSD: a Bayesian framework for parametric models of neural spectra
Source: arXiv:2410.20896 source file (2024-10-28)
Supplement: Supplementary file 1 [file appendix.tex]

\section{Bayesian methods}
        This section contains a brief introduction to approximate Bayesian inference and modern Bayesian approaches for mitigating competing hypothesis and group-level inference. It assumes no knowledge apart from basic probability theory. 
        \subsection{Bayes rule and Bayesian inversion}
            Let's assume that we are trying to model the distribution of some observed data $y$, governed by some parameters $\theta$. We usually come out with the functional form of the likelihood probability $p(y|\theta, m)$, i.e. the probability of the data $y$ given parameters $\theta$, under our model $m$. In the scope of this paper, we can think of the probability of an observed spectrum $y$ given the parameter of the periodic and aperiodic components $\theta$ under, for instance, a particular functional form of the spectral model $m$ assuming Gaussian peaks. In Bayesian statistics, we additionally reflect any prior knowledge about the parameters distribution by specifying their prior distribution, $p(\theta | $m$)$. The likelihood and prior completely determine the joint distribution of the data and parameters under our model, $p(y, \theta|m) = p(y|\theta, m) p(\theta | $m$)$.

            The main objective of Bayesian inference is two-folded. First, we want to refine our knowledge of the parameters distribution from the observed data. This implies that we want to compute the posterior probability $p(\theta |y, m)$, i.e. the parameter probability given the data, under our model. We can derive the posterior distribution by looking at the different factorisations of the joint distribution $p(y, \theta|m) = p(y|\theta, m) p(\theta | $m$) = p(\theta|y, m) p(y | $m$)$. Rearranging the terms yields Bayes rule:
            \begin{align}
                p(\theta|y,m) = \frac{p(y|\theta, m) p(\theta|m)}{p(y|m)}
            \end{align}
            This equation expresses the posterior distribution from the likelihood, the prior, and the marginal evidence $p(y|m)$. The second objective of Bayesian inference is to estimate the marginal evidence $p(y|m)$. This captures the probability of the data under a particular model, after accounting for the variability of -- i.e., integrating over -- all possible parameters:
            \begin{align}
                p(y| m) = \int p(y, \theta|m) d\theta
                \label{eq:marginal-evidence}
            \end{align}
            Computing the marginal and posterior distributions require to evaluate this crucial integral, which, in general, is computationally intractable due to the size of the parameter space. A computationally effective method to circumvent this problem is to use variational Bayesian methods, that we describe in the next section.   
            
        \subsection{Variational inference}
            Variational inference transforms the difficult problem of evaluating the integral \eqref{eq:marginal-evidence} by a simpler optimization problem. In variational Bayes, we seek to approximate the posterior distribution $p(\theta|y, m)$, which generally has an unfamiliar functional form, by a simpler parametric distribution $q_\phi(\theta)$. The approximate posterior $q_\phi(\theta)$ is chosen to have well known functional form, e.g., a multivariate Gaussian, parameterised by some parameters $\phi$, e.g., in the multivariate Gaussian case, its mean and covariance. In addition, we can make the approximate posterior factorise over a particular partition of the parameters, e.g, $q_\phi(\theta) = \prod_j q_\phi(\theta_{g_j})$, where each of the parameters is  mapped to one of the subset $g_j$. This is known as a mean field approximation and becomes important a bit later. 
            
            The core idea of variational Bayesian techniques is to refine the parameters $\phi$ to improve the estimate of the posterior distribution. To do so, we want to minimise an appropriate distance between $q_\phi(\theta)$ and $p(\theta|y, m)$. A natural choice is the Kullback-Leibler divergence: 
            \begin{align}
                D_{KL}(q_\phi(\theta) || p(\theta|y, m)) = - \int q_\phi(\theta) \ln \frac{ p(\theta|y, m)}{q_\phi(\theta)} d\theta
            \end{align}
            This divergence is a nice objective function as it is always positive and minimised whenever $ q_\phi(\theta) = p(\theta|y, m)$, but it directly involves the posterior and is thus intractable. However, we can use it to derive a tractable quantity. Looking at the inner quotient $ p(\theta|y, m)/{q_\phi(\theta)}$, we observe that multiplying both the numerator and denominator by $p(y, m)$ yields a new expression that involves the joint distribution $p(\theta, y|m)$ and the log marginal evidence $\ln p(y|m)$:
            \begin{align}
                D_{KL}(q_\phi(\theta) || p(\theta|y, m)) = - \int q_\phi(\theta) \ln \frac{ p(\theta,y| m)}{q_\phi(\theta)} d\theta + \ln p(y|m)
                \label{eq:kl-divergence}
            \end{align}
            Let's denote the new integral quantity $F_m[q_\phi]$:
            \begin{align}
                 F_m[q_\phi] = \int q_\phi(\theta) \ln \frac{ p(\theta,y| m)}{q_\phi(\theta)} d\theta
                 \label{eq:free-energy}
            \end{align} 
            This quantity depends only on the approximate posterior $q_\phi$, which we easily evaluate for a particular value of $\phi$, and on the joint distribution $p(y, \theta|m)$, which we specify through the likelihood $p(y|\theta,m)$ and the prior $p(\theta|m)$. In particular, this formulation holds for any choice of $q_\phi$. Thus, even if the integration in \eqref{eq:free-energy} is conducted over the same high dimensional space as that of \eqref{eq:marginal-evidence}, we are now free to select any particular form of the approximate posterior that would help simplify the integral. We will see later that a Gaussian approximate posterior is a convenient choice as it enables using Laplace approximation. For now, we want to grasp how this new quantity can be useful for Bayesian inference. 
            
            Rearranging the terms in \eqref{eq:kl-divergence}, we have 
            \begin{align}
                 F_m[q_\phi] = \ln p(y|m) -  D_{KL}(q_\phi(\theta) || p(\theta|y, m)) \leq \ln p(y|m)
                 \label{eq:free-energy}
            \end{align} 
            where the last inequality comes from the positivity of the KL divergence.  Thus, for any $q_\phi$, we have derived a quantity $F_m[q_\phi]$ that is always smaller or equal to the log marginal evidence of the model, $\ln p(y|m)$, with equality whenever the  approximate posterior $q_\phi(\theta)$ equals the true posterior $p(\theta|y, m)$. From now on, we refer to this quantity $F_m[q_\phi]$ as the variational free-energy (VFE), although it is also called Evidence Lower Bound (ELBO) in machine learning. 

            The objective of variational Bayes method is to find the optimal parameters $\phi^*$ that maximises the VFE, or formally, to solve the following unconstrained optimisation problem
            \begin{align}
                \phi^* = \arg \max_\phi F_m[q_\phi]
            \end{align}
            We can consider using an iterative procedure such as gradient ascent to maximise the VFE. Interestingly, convergence occurs whenever we have minimised the KL divergence, i.e., when the approximate posterior is as close as it can be to the true posterior, which for any model that is expressive enough, implies 
             \begin{align}
                 q_{\phi^*}(\theta) \approx p(\theta|y,m)
             \end{align}
            In that case, it is safe to assume that the KL divergence is small as compared to the log evidence.  This assumption leads to the following approximation
            \begin{align}
                F_m[q_{\phi^*}] \approx \ln p(y|m) 
            \end{align}

            To summarise, resorting to variational inference, we have constructed a variational free-energy which depends on the approximate posterior $q_\phi$ and is a lower bound on the log evidence. We have observed that by maximising the free-energy, we obtain an approximation of the two quantity of interest for Bayesian inference: a good approximation of the true posterior, $q_{\phi^*}(\theta) \approx p(\theta|y,m)$, and a good approximation of the (log-) model evidence,  $F_m[q_{\phi^*}] \approx \ln p(y|m)$. Thus, we have casted the difficult problem of Bayesian inference as an optimisation problem, for which we can solve using any gradient descent algorithm. In the next section, we will see how the difference in variational free-energy between different models can be used to mitigate between competing hypotheses.             
        \subsection{Bayesian model comparison}
            Let say that we have two competing hypotheses, $H_1$ and $H_2$, that we can translate into two models $m_1$ and $m_2$, for which we prescribe a joint distribution of data and parameters $p(y, \theta|m_1)$ and $p(y, \theta|m_2)$. Having observed some data $y$, we want to assess whether one hypothesis is more likely than the other given the data. Formally, if $H_1$ is $k$ times more probable than $H_2$ after observing $y$, we would simply write $p(m_1|y) = k \, p(m_2|y)$. This factor $k$, intuitive and helpful for arbitrating between two competing hypothesis, is called the Bayes factor. Interestingly,  if we assume that both hypotheses are equiprobable a priori, i.e. $p(m_1) = p(m_2)$, we can apply Bayes rule to obtain
            \begin{align}
                k = \frac{p(m_1|y)}{p(m_2|y)} = \frac{p(y|m_1) p(m_1)}{p(y|m_2)p(m_2)} = \frac{p(y|m_1)}{p(y|m_2)} 
            \end{align}
            Let us unpack this equation: the Bayes factor between two equiprobable hypotheses is simply the ratio of the marginal evidence of probabilistic models of these hypotheses. In other words, mitigating between hypotheses amounts to constructing their probabilistic models and comparing their ability to predict the data. 
            
            We can even go one step further and notice that the marginal evidence is the likelihood of the data under a model; hence, the Bayes factor is a likelihood ratio. By the Neyman-Pearson lemma, mitigating between hypothesis using a likelihood ratio is the most powerful (i.e., sensitive) test across all possible levels of specificity. In other words, for Bayesian model comparison, using the Bayes factor as a decision criterion maximises the Area Under the Curve (AUC) of the Receiver Operating Characteristic (ROC) curve.

            Within the context of variational inference, the marginal evidence is approximated by the variational free-energy. Dropping references to the approximate posterior for brevity, we can write the log Bayes factor between two models as: 
            \begin{align}
                \ln k \approx F_{m_1} - F_{m_2}
                \label{eq:log-bf}
            \end{align}
            At this point, we must mention a subtlety  about the approximation in \eqref{eq:log-bf}. This approximation can hold independently of the validity of $F_{m_1} \approx \ln p(y|m_1)$ or $F_{m_2} \approx \ln p(y|m_2)$: it simply requires that both approximate posteriors are as close to the true posteriors, such as the difference in KL divergences is negligible as compared to the difference in log evidence. 
        \subsection{Bayesian model reduction}
        \subsection{Parametric empirical Bayes}
